# Supplementary material for: Interplay of phase boundary anisotropy and electro-autocatalytic surface reactions on the lithium intercalation dynamics in Li$_X$FePO$_4$ platelet-like nanoparticles
Source: arXiv:1802.05847 source file (2018-02-16)
Supplement: Supplementary file 1 [file SupplementaryMaterials.pdf]

# Supplementary materials for
# Interplay of phase boundary anisotropy and electro-autocatalytic surface reactions on the lithium intercalation dynamics in $Li_X FePO_4$ platelet-like nanoparticles

Neel Nadkarni[1], Elisha Rejovitzky[1], Dimitrios Fraggedakis[1], Claudio V. Di Leo[2], Raymond B. Smith[1], Peng Bai[3], and Martin Z. Bazant[1,4]
[1] *Department of Chemical Engineering, Massachusetts Institute of Technology, Cambridge, MA 02139, USA*
[2] *School of Aerospace Engineering, Georgia Institute of Technology, Atlanta, GA 30332, USA*
[3] *Department of Energy, Environment, and Chemical Engineering, Washington University at St. Louis, MO 63130, USA and*
[4] *Department of Mathematics, Massachusetts Institute of Technology, Cambridge, MA 02139, USA*

## I. LIST OF MATERIAL PARAMETERS

Here is the list of the material parameters used for our computations.

Table I. List of material parameters

| Parameter | Physical meaning | Value | Units | Source |
|---|---|---|---|---|
| $T$ | Temperature | 298 | K | |
| $c_{\max}$ | Max. conc. | $2.29\times10^4$ | mol/m$^3$ | [1] |
| $\Omega$ | Partial molar vol. | $11.2\times10^3$ | J/mol | [2] |
| $\kappa_x$ | | 0.022 | J$\mu$m$^2$/mol | [1, 2] |
| $\kappa_y$ | Interfacial tension | 2.2 | J$\mu$m$^2$/mol | [1–3] |
| $\kappa_z$ | | 0.022 | J$\mu$m$^2$/mol | [1, 2] |
| $\Delta\gamma_{ac}$ | | 0.26 | J/m$^2$ | [4] |
| $\Delta\gamma_{ab}$ | Surface energy | 0.26 | J/m$^2$ | |
| $\Delta\gamma_{bc}$ | | -0.4 | J/m$^2$ | |
| $C_{11}$ | | 157.4 | | |
| $C_{22}$ | | 175.8 | | |
| $C_{33}$ | | 154 | | |
| $C_{44}$ | Elastic stiffness [a] | 37.8 | GPa | |
| $C_{55}$ | | 49.05 | | [5] |
| $C_{66}$ | | 51.6 | | |
| $C_{12}$ | | 51.2 | | |
| $C_{13}$ | | 53.25 | | |
| $C_{23}$ | | 32.7 | | |
| $\epsilon^0_{aa}$ | | 0.05 | | |
| $\epsilon^0_{bb}$ | Chemical strain | 0.028 | | |
| $\epsilon^0_{cc}$ | | -0.025 | | |
| $D_a$ | | $10^{-14}$ | | |
| $D_b$ | Diffusivity | $10^{-9}$ | cm$^2$/s | [6] |
| $D_c$ | | $10^{-14}$ | | |
| $k$ | Reaction rate [b] | $10^{-3}$ | A/m$^2$ | [7–9] |

[a] Stiffness indices follow Voigt notations, i.e., {1, 2, 3, 4, 5, 6} map into {*aa*, *bb*, *cc*, *bc*, *ac*, *ab*}. The Stiffness values are averaged from the $FePO_4$ and $LiFePO_4$ values.
[b] Value was modified to account for the reduction in active reaction surface due to the highly inhomogeneous lithiation patterns.

## II. SPATIAL AVERAGING PROCESS

The amount of phase separation that has occurred in the particle is quantified using a spatial average given by

$$\langle (c-X)^2 \rangle = \frac{1}{V}\int_V |c-X|^2\, dV. \tag{1}$$

In our analysis, we wish to study the effects of the surface reactions on the phase separation in the bulk. Therefore, we choose an area smaller than the particle size, sufficiently within the bulk so that the surface properties do not affect the averaged value. The area utilized for spatial averaging is shown in Fig. 1.

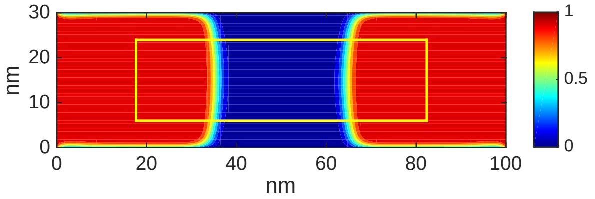


Figure 1. An example simulation showing the averaging technique. The spatial averaging is performed over the area of the box outlined by the yellow lines.

## III. SPECIMEN PREPARATION

The initial condition for the lithiation simulations is a particle at its pre-lithiated state with the wetted/ dewetted surfaces and accompanying stresses. In order to compute this initial condition with a low computational cost, we designed a specimen preparation scheme that transitions through simple morphologies. We performed a simulation which begins at a reference configuration of an almost empty stress-free particle with a uniform concentration of $\bar{c} = 0.05$ and no surface wetting energy. For the studied cases of dewetted and neutral ac facets, the concentrations at the side facets were ramped to full wetting conditions, and the surface energies of top and bottom facets were ramped to their respective values resulting in a quick transition to a morphology similar to the one we require. Then, the Dirichlet boundary conditions on the

concentration at the side facets were switched to Neumann boundary conditions for the surface energy and the particle was left to relax. During this process, the species exchange through diffusion and reaction caused deformations and stresses. The resulting concentration profile is presented in Fig. 1A of the main paper.

## IV. EQUILIBRIUM PROFILE IN THE CASE OF PARTIAL LITHIATION

For half-lithiated particles ($\langle \bar{c} \rangle = X = 0.5$), the morphology slowly evolves to reduce elastic energy by removing the interface parallel to the $a$-axis. Fig. 2 presents the concentration profile that develops after stopping lithiation at the state described in Fig. 3C of the main paper and letting the nanoparticle relax for 60 min. During the relaxation time, significant lithium exchange between the Li-channels occurs through reaction and $a$-axis diffusion. The resulting morphology reduces the interface normal to the $b$-axis in exchange for preferable $a$-axis interfaces, and reduces the overall length of the interfaces to minimize the free energy.

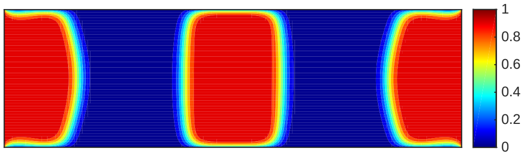


Figure 2. An equilibrium concentration profile in the nanoparticle 60min after pausing a lithiation of a 1C rate at SOC = 0.5.


[1] P. Bai, D. A. Cogswell, and M. Z. Bazant, Nano letters **11**, 4890 (2011).

[2] D. A. Cogswell and M. Z. Bazant, ACS nano **6**, 2215 (2012).

[3] N. Ohmer, B. Fenk, D. Samuelis, C.-C. Chen, J. Maier, M. Weigand, E. Goering, and G. Schütz, Nature communications **6**, 6045 (2015).

[4] L. Wang, F. Zhou, Y. Meng, and G. Ceder, Physical Review B **76**, 165435 (2007).

[5] T. Maxisch and G. Ceder, Physical Review B **73**, 174112 (2006).

[6] R. Malik, D. Burch, M. Bazant, and G. Ceder, Nano letters **10**, 4123 (2010).

[7] P. Bai and M. Bazant, Nature communications **5**, 3585 (2014).

[8] J. Lim, Y. Li, D. H. Alsem, H. So, S. C. Lee, P. Bai, D. A. Cogswell, X. Liu, N. Jin, Y.-s. Yu, N. J. Salmon, D. A. Shapiro, M. Z. Bazant, T. Tyliszczak, and W. C. Chueh, Science **353**, 566 (2016).

[9] X. Zhang, M. Van Hulzen, D. P. Singh, A. Brownrigg, J. P. Wright, N. H. Van Dijk, and M. Wagemaker, Nature communications **6** (2015).
